# Supplementary material for: Conv-MPN: Convolutional Message Passing Neural Network for Structured Outdoor Architecture Reconstruction
Source: arXiv:1912.01756 source file (2021-06-07)
Supplement: Supplementary file 1 [file appendix_IP_paper.tex]

% \section{Additional Reference}
% In our paper, we cite a CVPR2020 submitted paper. The anonymized version of the paper is shown after all the additional qualitative results.

\setcounter{section}{0}
\setcounter{figure}{0}
\setcounter{table}{0}

\twocolumn[{
   {
   \newpage
   \null
   \vskip .375in
   \begin{center}
      {\Large \bf Vectorizing World Buildings: Planar Graph Inference via Deep Neural Networks and Integer Programming \par}
      % additional two empty lines at the end of the title
      \vspace*{24pt}
      {
      \large
      \lineskip .5em
      \begin{tabular}[t]{c}
         \ifcvprfinal\@author\else Anonymous CVPR submission\\
         %\vspace*{1pt}\\%This space will need to be here in the final copy, so don't squeeze it out for the review copy.
%Paper ID \cvprPaperID 
        \fi
      \end{tabular}
      \par
      }
      % additional small space at the end of the author name
      \vskip .5em
      % additional empty line at the end of the title block
      \vspace*{12pt}
   \end{center}
   }
%\vspace{-2em}
\centerline{
\includegraphics[width=\linewidth]{IP_images/new_teaser.pdf}
}
\captionof{figure}{
The paper takes a RGB image, detects three geometric primitives (i.e., corners, edges, and regions), classifiers their relationships (i.e., corner-to-edge and region-to-region), and fuses the information via Integer Programming to reconstruct a planar graph.}
\label{fig:teaser}
\vspace{1em}
}]
\input{IP_sections/0_abstract.tex}
\input{IP_sections/1_introduction.tex}
\input{IP_sections/2_related_work.tex}
\input{IP_sections/3_problem.tex}
\input{IP_sections/4_method.tex}
\input{IP_sections/5_experimental_results.tex}
\input{IP_sections/6_conclusion.tex}

\clearpage
{\small
\bibliographystyle{ieee_fullname}
\bibliography{IP_egbib}
}
