# Supplementary material for: Conv-MPN: Convolutional Message Passing Neural Network for Structured Outdoor Architecture Reconstruction
Source: arXiv:1912.01756 source file (2021-06-07)
Supplement: Supplementary file 2 [file appendix_architecture.tex]

\section{Neural architecture specifications}
Table~\ref{table:Conv-MPN} shows the full specification of the three neural modules constituting the Conv-MPN architecture. %Specifically, We set $t_1=1,2,3;t_2=0$. $t_1=3$ shows the best results.
%
%\fuyang{we use two ways to describe the Architectures of Conv-MPN, GNN. We can't decide which one to use. For table \ref{table:architecture}, we attempt to describe Conv-MPN and GNN in one table. For table \ref{table:Conv-MPN} and table \ref{table:gnn}, we split Conv-MPN, gnn into two tables. }
In the comparative evaluations, we used a vanilla graph neural network as a baseline, whose specification is given in Table~\ref{table:gnn}.

\begingroup

\begin{table*}[!h]
\caption{Conv-MPN architecture specification. For the feature initialization module, the three blocks are initialized with the first three blocks of DRN-C-26, which was pretrained on the ImageNet. We max-pool features of all the neighbor nodes and concatenate it with node feature as input of the message passing. $[\cdot]$ represents residual block. $\cdot\} \times i$ denotes repeating the layers i times. $t$ denotes number of convolutional message passing iterations.}
\label{table:Conv-MPN}
\centering
\begin{tabular}{lccc}
\toprule
Module & Stage & Specification & Output Size\\
\midrule
\midrule
Feature initialization & $conv\_relu\_bn_1$ & $4\times7\times7,16, stride=1$ &  $16\times256\times256$\\
\cmidrule{2-4}
&$residual\_block_1$& ${
\left[ \begin{array}{c}
16\times3\times3, 16, stride=1\\
16\times3\times3, 16, stride=1\\
\end{array} 
\right ]}\times1$ & $16\times256\times256$\\
\cmidrule{2-4}
&$residual\_block_2$& ${
\left[ \begin{array}{c}
16\times3\times3, 32, stride=2\\
32\times3\times3, 32, stride=1\\
\end{array} \right ]}
\times1$& $32\times128\times128$\\
\cmidrule{2-4}
&$residual\_block_3$& ${
\left[ \begin{array}{c}
32\times3\times3, 64, stride=2\\
64\times3\times3, 64, stride=1\\
\end{array} \right ]}\times2$& $64\times64\times64$\\
\cmidrule{2-4}
&$conv\_relu\_bn_2$&$64\times3\times3,32,stride=1$ & $32\times64\times64$\\
\midrule
Convolutional message passing & $\begin{array}{c}
conv\_relu\_bn_3\\
conv\_relu\_bn_4\\
conv\_relu\_bn_5\\
\end{array}$&${
\left . \begin{array}{c}
{\left . \begin{array}{c}
64\times3\times3, 64, stride=1
\end{array} \right \}}\times 4 \\
{\left . \begin{array}{c}
64\times3\times3, 32, stride=1
\end{array} \right \}}\times 1 \\
{\left . \begin{array}{c}
32\times3\times3, 32, stride=1
\end{array} \right \}}\times 2 \\
\end{array} \right \}}\times t$ & $32\times64\times64$\\
\midrule
Building edge verification &  $\begin{array}{c}
conv\_relu\_bn_6\\
conv\_relu\_bn_7\\
conv\_relu\_bn_8\\
conv\_relu\_bn_9\\
conv\_relu\_bn_{10}\\
\end{array}$ & 
$
\begin{array}{r}
32\times3\times3, 32, stride=1\\
32\times3\times3, 64, stride=1\\
64\times3\times3, 64, stride=1\\
64\times3\times3, 128, stride=1\\
128\times3\times3, 128, stride=1\\
\end{array}
$ & $128\times64\times64$ \\
\cmidrule{2-4}
& $max\_pooling$ & $32\times32, max, stride=32$& $128\times2\times2$ \\
\cmidrule{2-4}
& $fc$ & $512\times2$ & 2 \\
\bottomrule
\end{tabular}
\end{table*}
\endgroup

\begingroup

\begin{table*}[!h]
\caption{The architecture specification of Vanilla GNN, a baseline method in our comparative evaluations. The feature initialization module encodes each building edge into a 512d vector instead of a feature volume.
%For the feature initialization module, the architecture is same with Feature initialization + Building edge verification (before max-pooling) in Conv-MPN. After max-pooling layer, the feature is flatten into 512 1d vector. 
The message passing module max-pools all the neighboring nodes and concatenate the pooled vector to generate an input of the fully connected layer. $[\cdot]$ represents residual block. $\cdot\} \times i$ denotes repeating the layers i times. $t$ denotes number of vanilla message passing iterations.}
\label{table:gnn}
\centering
\begin{tabular}{lccc}
\toprule
Module & Stage & Specification & Output Size\\
\midrule
\midrule
Feature initialization & $conv\_relu\_bn_1$ & $4\times7\times7,16, stride=1$ &  $16\times256\times256$\\
\cmidrule{2-4}
&$residual\_block_1$& ${
\left[ \begin{array}{c}
16\times3\times3, 16, stride=1\\
16\times3\times3, 16, stride=1\\
\end{array} 
\right ]}\times1$ & $16\times256\times256$\\
\cmidrule{2-4}
&$residual\_block_2$& ${
\left[ \begin{array}{c}
16\times3\times3, 32, stride=2\\
32\times3\times3, 32, stride=1\\
\end{array} \right ]}
\times1$& $32\times128\times128$\\
\cmidrule{2-4}
&$residual\_block_3$& ${
\left[ \begin{array}{c}
32\times3\times3, 64, stride=2\\
64\times3\times3, 64, stride=1\\
\end{array} \right ]}\times2$& $64\times64\times64$\\
\cmidrule{2-4}
&$\begin{array}{c}
conv\_relu\_bn_2\\
conv\_relu\_bn_3\\
conv\_relu\_bn_4\\
conv\_relu\_bn_5\\
conv\_relu\_bn_6\\
conv\_relu\_bn_7\\
\end{array}$ & 
$
\begin{array}{r}
64\times3\times3,32,stride=1\\
32\times3\times3, 32, stride=1\\
32\times3\times3, 64, stride=1\\
64\times3\times3, 64, stride=1\\
64\times3\times3, 128, stride=1\\
128\times3\times3, 128, stride=1\\
\end{array}
$ & $128\times64\times64$ \\
\cmidrule{2-4}
& $max\_pooling$ & $32\times32, max, stride=32$& $128\times2\times2$ \\
\midrule
Message passing &
$\begin{array}{c}
fc\_relu\_bn_8\\
fc\_relu\_bn_9\\
fc\_relu\_bn_{10}\\
\end{array}$ & 
${
\left . \begin{array}{c}
{\left . \begin{array}{c}
1024\times1024
\end{array} \right \}}\times 3 \\
{\left . \begin{array}{c}
1024\times512
\end{array} \right \}}\times 1 \\
{\left . \begin{array}{c}
512\times512
\end{array} \right \}}\times 2 \\
\end{array} \right \}}\times t$
& $512$ \\
\midrule
& $fc$ & $512\times2$ & 2 \\
\bottomrule
\end{tabular}
\end{table*}
\endgroup
