# Supplementary material for: Conv-MPN: Convolutional Message Passing Neural Network for Structured Outdoor Architecture Reconstruction
Source: arXiv:1912.01756 source file (2021-06-07)
Supplement: Supplementary file 3 [file appendix_graph_generation.tex]

\section{Training data preparation} \label{grah_gneration}
Conv-MPN requires building corner detection as a pre-processing, making it impossible to generate a ground-truth planar graph when some corners are missed. Therefore, we generate two sets of training data, one using ground-truth corners and the other using detected corners. We trained Conv-MPN (and its variants) by alternating these two sets of training data until convergence.
%
%During training, we generate two sets of target building graphs, i.e. 
%one derived from ground-truth annotations and the other built upon detected corners using a heuristic (See Figure \ref{fig:heuristic_graph_match}). In short, we train Conv-MPN and variants, alternating on both sets until reaching convergence. This procedure led to best performance. Next, we provide more details on how we obtain each target graph set.

\mysubsubsection{From ground-truth corners} 
We use the ground-truth building corners and the planar-graph as the input and output of Conv-MPN.
%Since annotations are provided as a planar graph, we can directly utilize these graphs as target however, 
We added small perturbations (i.e. $\mathcal{N}(0, 2^{2})$ to corner $(x, y)$ coordinates for better generalization.
% Annotated graph is simple, which is generated from the ground-truth annotation. Specifically, we have ground-truth corners and ground-truth edges which can be represented by a pair of ground-truth corners. We use the ground-truth corners added with Gaussian noise($\mu=0$, $\sigma=2$) to generate the annotated graph. Every pair of corners are represented as a node in the annotated graph (See Fig. 2 in the original submission%\ref{fig:preprocessing}
% ). The nodes are labeled as True if and only if the corresponding building-edges are true.

\mysubsubsection{From detected corners} Target corners are determined by assigning each detected corner candidate to the closest ground-truth corner as long as they are within 7 pixels distant from each other. Now, considering every pair of detected corners, we utilize the corner detection and annotation assignment to derive positive and negative targets for edges. A candidate edge is set to be positive if (1) its end-points map to an edge in the annotations or (2) if there is corner that is colinear and a common neighbour to its end-points. Worth to mention that we only apply the latter case, if the annotated colinear corner is not assigned to any other detected corner (otherwise we would be allowing duplicated colinear edges). For all other cases not in (1) or (2), the candidate edge is set to be a negative target.

% \begin{itemize}
%     \item a. For a given edge 
    
%     one of the corners of $p_i$ or $p_j$ is not matched with ground-truth corners, then $(p_i, p_j)$ is set to false.
%     \item b. Both $p_i$ and $p_j$ are matched with ground-truth corners $\hat{p_k}$ and $\hat{p_l}$ respectively. If $(\hat{p_k}, \hat{p_l})$ is true edge in the ground-truth edges set, then $(p_i, p_j)$ is set to true as well.
%     \item c. Otherwise, if $(\hat{p_k}, \hat{p_l})$ is not in the ground-truth edges set, we iterate all the neighbors of $\hat{p_k}$(also for $\hat{p_l}$) that not matched with a detected corner. If $\hat{p_l}$ is neighbor of one of those unmatched corners, $\hat{p_m}$, and direction of $\overrightarrow{\hat{p_m}\hat{p_l}}$ and $\overrightarrow{\hat{p_k}\hat{p_m}}$ are equal, then we set $(p_i, p_j)$ to true.
% \end{itemize}

% 1. match all the ground-truth corners with nearest detected corners.
% $$
%     m_i = \mathop{\arg\min}_{j} \ \| \hat{p_i} - p_j\|.
% $$
% where $m_i$ is the index of the nearest detected corners with ground-truth corner $\hat{p_i}$. If the $\mathcal{L}_2$-distance of $\hat{p_i}$ and $p_{m_i}$ less than threshold $\eta$, then the ground-truth corner $\hat{p_i}$ and $p_{m_i}$ are matched, otherwise, $\hat{p_i}$ is not matched with detected corners.

% 2. we set each pair of detected corners $(p_i, p_j)$ as true or false based on the following rules (See Fig. \ref{fig:heuristic_graph_match}):

\begin{figure}
    \centering
    \includegraphics[width=0.7\linewidth]{images/heuristic_graph_match.pdf}
    \caption{
    Illustration of a sample training data preparation process. The red shows the ground-truth planar graph. The blue 
    %how target graphs generated from annotations and in blue target 
    shows the one generated from detected corners.
    %a building graph, built from detected corners. 
    Even with missed building corners, the process is able to generate a reasonable building graph.
    %Note that for the simple case where we miss one colinear corner, our heuristics still build a reasonable graph and set edge $e_3$ and $e_4$ as a positive target. 
    % Red circles represent the ground-truth corners, red lines represent ground-truth edges. Blue circles represent the detected corners, and blue lines represent the true edges followed by the matching rules. The $e_1, e_2$ are selected based on rule b, and $e_3, e_4$ are selected based on rule c.
    }
    \label{fig:heuristic_graph_match}
\end{figure}
