# Supplementary material for: Conv-MPN: Convolutional Message Passing Neural Network for Structured Outdoor Architecture Reconstruction
Source: arXiv:1912.01756 source file (2021-06-07)
Supplement: Supplementary file 4 [file appendix_results.tex]

\section{Additional experimental results}
Figures~\ref{fig:results_0}-~\ref{fig:results_34} show additional experimental results with the six baseline methods over all testing samples.

\begin{figure*}
\centering
\includegraphics[width=\linewidth]{results_compress/grid_im_0.jpg}
\caption{Additional qualitative results.}
\label{fig:results_0}
\end{figure*}

\begin{figure*}
\centering
\includegraphics[width=\linewidth]{results_compress/grid_im_1.jpg}
\caption{Additional qualitative results.}
\label{fig:results_1}
\end{figure*}

\begin{figure*}
\centering
\includegraphics[width=\linewidth]{results_compress/grid_im_2.jpg}
\caption{Additional qualitative results.}
\label{fig:results_2}
\end{figure*}

\begin{figure*}
\centering
\includegraphics[width=\linewidth]{results_compress/grid_im_3.jpg}
\caption{Additional qualitative results.}
\label{fig:results_3}
\end{figure*}

\begin{figure*}
\centering
\includegraphics[width=\linewidth]{results_compress/grid_im_4.jpg}
\caption{Additional qualitative results.}
\label{fig:results_4}
\end{figure*}

\begin{figure*}
\centering
\includegraphics[width=\linewidth]{results_compress/grid_im_5.jpg}
\caption{Additional qualitative results.}
\label{fig:results_5}
\end{figure*}

\begin{figure*}
\centering
\includegraphics[width=\linewidth]{results_compress/grid_im_6.jpg}
\caption{Additional qualitative results.}
\label{fig:results_6}
\end{figure*}

\begin{figure*}
\centering
\includegraphics[width=\linewidth]{results_compress/grid_im_7.jpg}
\caption{Additional qualitative results.}
\label{fig:results_7}
\end{figure*}

\begin{figure*}
\centering
\includegraphics[width=\linewidth]{results_compress/grid_im_8.jpg}
\caption{Additional qualitative results.}
\label{fig:results_8}
\end{figure*}

\begin{figure*}
\centering
\includegraphics[width=\linewidth]{results_compress/grid_im_9.jpg}
\caption{Additional qualitative results.}
\label{fig:results_9}
\end{figure*}

\begin{figure*}
\centering
\includegraphics[width=\linewidth]{results_compress/grid_im_10.jpg}
\caption{Additional qualitative results.}
\label{fig:results_10}
\end{figure*}

\begin{figure*}
\centering
\includegraphics[width=\linewidth]{results_compress/grid_im_11.jpg}
\caption{Additional qualitative results.}
\label{fig:results_11}
\end{figure*}

\begin{figure*}
\centering
\includegraphics[width=\linewidth]{results_compress/grid_im_12.jpg}
\caption{Additional qualitative results.}
\label{fig:results_12}
\end{figure*}

\begin{figure*}
\centering
\includegraphics[width=\linewidth]{results_compress/grid_im_13.jpg}
\caption{Additional qualitative results.}
\label{fig:results_13}
\end{figure*}

\begin{figure*}
\centering
\includegraphics[width=\linewidth]{results_compress/grid_im_14.jpg}
\caption{Additional qualitative results.}
\label{fig:results_14}
\end{figure*}

\begin{figure*}
\centering
\includegraphics[width=\linewidth]{results_compress/grid_im_15.jpg}
\caption{Additional qualitative results.}
\label{fig:results_15}
\end{figure*}

\begin{figure*}
\centering
\includegraphics[width=\linewidth]{results_compress/grid_im_16.jpg}
\caption{Additional qualitative results.}
\label{fig:results_16}
\end{figure*}

\begin{figure*}
\centering
\includegraphics[width=\linewidth]{results_compress/grid_im_17.jpg}
\caption{Additional qualitative results.}
\label{fig:results_17}
\end{figure*}

\begin{figure*}
\centering
\includegraphics[width=\linewidth]{results_compress/grid_im_18.jpg}
\caption{Additional qualitative results.}
\label{fig:results_18}
\end{figure*}

\begin{figure*}
\centering
\includegraphics[width=\linewidth]{results_compress/grid_im_19.jpg}
\caption{Additional qualitative results.}
\label{fig:results_19}
\end{figure*}

\begin{figure*}
\centering
\includegraphics[width=\linewidth]{results_compress/grid_im_20.jpg}
\caption{Additional qualitative results.}
\label{fig:results_20}
\end{figure*}

\begin{figure*}
\centering
\includegraphics[width=\linewidth]{results_compress/grid_im_21.jpg}
\caption{Additional qualitative results.}
\label{fig:results_21}
\end{figure*}

\begin{figure*}
\centering
\includegraphics[width=\linewidth]{results_compress/grid_im_22.jpg}
\caption{Additional qualitative results.}
\label{fig:results_22}
\end{figure*}

\begin{figure*}
\centering
\includegraphics[width=\linewidth]{results_compress/grid_im_23.jpg}
\caption{Additional qualitative results.}
\label{fig:results_23}
\end{figure*}

\begin{figure*}
\centering
\includegraphics[width=\linewidth]{results_compress/grid_im_24.jpg}
\caption{Additional qualitative results.}
\label{fig:results_24}
\end{figure*}

\begin{figure*}
\centering
\includegraphics[width=\linewidth]{results_compress/grid_im_25.jpg}
\caption{Additional qualitative results.}
\label{fig:results_25}
\end{figure*}

\begin{figure*}
\centering
\includegraphics[width=\linewidth]{results_compress/grid_im_26.jpg}
\caption{Additional qualitative results.}
\label{fig:results_26}
\end{figure*}

\begin{figure*}
\centering
\includegraphics[width=\linewidth]{results_compress/grid_im_27.jpg}
\caption{Additional qualitative results.}
\label{fig:results_27}
\end{figure*}

\begin{figure*}
\centering
\includegraphics[width=\linewidth]{results_compress/grid_im_28.jpg}
\caption{Additional qualitative results.}
\label{fig:results_28}
\end{figure*}

\begin{figure*}
\centering
\includegraphics[width=\linewidth]{results_compress/grid_im_29.jpg}
\caption{Additional qualitative results.}
\label{fig:results_29}
\end{figure*}

\begin{figure*}
\centering
\includegraphics[width=\linewidth]{results_compress/grid_im_30.jpg}
\caption{Additional qualitative results.}
\label{fig:results_30}
\end{figure*}

\begin{figure*}
\centering
\includegraphics[width=\linewidth]{results_compress/grid_im_31.jpg}
\caption{Additional qualitative results.}
\label{fig:results_31}
\end{figure*}

\begin{figure*}
\centering
\includegraphics[width=\linewidth]{results_compress/grid_im_32.jpg}
\caption{Additional qualitative results.}
\label{fig:results_32}
\end{figure*}

\begin{figure*}
\centering
\includegraphics[width=\linewidth]{results_compress/grid_im_33.jpg}
\caption{Additional qualitative results.}
\label{fig:results_33}
\end{figure*}

\begin{figure*}
\centering
\includegraphics[width=\linewidth]{results_compress/grid_im_34.jpg}
\caption{Additional qualitative results.}
\label{fig:results_34}
\end{figure*}

%\begin{figure*}
%\centering
%\includegraphics[width=\linewidth]{results_compress/grid_im_35.jpg}
%\caption{Additional qualitative results.}
%\label{fig:results_35}
%\end{figure*}
